# Supplementary material for: Trajectory Mamba: Efficient Attention-Mamba Forecasting Model Based on Selective SSM
Source: arXiv:2503.10898 source file (2025-03-13)
Supplement: Supplementary file 1 [file X_suppl.tex]

\clearpage
\setcounter{page}{1}
\maketitlesupplementary

\section{More Comparison with State of the Art}
\label{sec:rationale}
In the supplementary materials, we further assess the effectiveness of Tamba. Specifically, we manually reproduced the methods marked with “-" in the parameter column of table \ref{tab:ag1}. Additionally, we use FLOPs(G) as a metric to assess the computational complexity of listed models. To ensure a fair comparison, we conducted all experiments under the same environment (batch size, epochs, etc.) using eight NVIDIA 3090TI GPUs ensuring that factors such as memory, data transfer, and hardware optimizations did not introduce unfairness.

\begin{figure*}
    \centering
    \includegraphics[width=\linewidth]{Trajectory Mamba/Images/img4.pdf}
    \caption{More qualitative results on the Argoverse 2 validation set. We conduct four different traffic scenarios. (a). Multi-agents in straight-road scenario, (b). Multiple agents on roundabout road, (c). Vehicle avoidance after roundabout, (d). Mixed scenario involving pedestrians and vehicles.}
    \label{fig:5}
\end{figure*}

\begin{table*}[t]
\scriptsize
\centering
\fontsize{9pt}{11pt}\selectfont
\tabcolsep=0.15cm

\begin{tabular}{c|cccc|ccc|cc}
\hline
Method & \textbf{b-minFDE$_{6}$}$\downarrow$ &minADE$_{6}$$\downarrow$ & minFDE$_{6}$$\downarrow$ & MR$_{6}$$\downarrow$ & minADE$_{1}$$\downarrow$ & minFDE$_{1}$$\downarrow$ & MR$_{1}$$\downarrow$ & Params (M)$\downarrow$& FLOPs(G)$\downarrow$ \\
\hline
THOMAS \cite{gilles2022thomas} & 2.16 & 0.88 & 1.51 & 0.20 & 1.95 & 4.71 & 0.64 & - & -\\
GoRela \cite{cui2023gorela} & 2.01 & 0.76 & 1.48 & 0.22 & 1.82 & 4.62 & 0.66 & - & -\\
QML \cite{su2022qml} & 1.95 & 0.69 & 1.39 & 0.19 & 1.84 & 4.98 & 0.62 & 9.39 & -\\
MTR \cite{shi2024mtr++} & 1.98 & 0.73 & 1.44 & 0.15 & 1.74 & 4.39 & 0.58 & 65.78  & - \\
GANet \cite{wang2023ganet} & 1.96 & 0.72 & 1.34 & 0.17 & 1.77 & 4.48 & 0.59 & 61.73  & 15.79 \\
BANet \cite{wang2023technical} & 1.92 & 0.71 & 1.36 & 0.19 & 1.79 & 4.61 & 0.60 & 9.49  & \textbf{11.93} \\
QCNet \cite{zhou2023query} & 1.91 & 0.65 & 1.29 & \textbf{0.16} & 1.69 & 4.30 & 0.59 & 7.66 & 45.3\\
\hline
\textbf{Tamba (Ours)} & \textbf{1.89} & \textbf{0.64} & \textbf{1.24} &0.17 & \textbf{1.66} & \textbf{4.24} & \textbf{0.57} & \textbf{4.54} & 27.3\\
\hline
\end{tabular}
\caption{Performance comparison on Argoverse 2 \cite{Argoverse2, TrustButVerify} dataset, leaderboard ranked by b-minFDE$_{6}$. Subscript $_{6}$ and $_{1}$ represents the number of predictions; baselines are marked using the symbol "*". For each metric, best performance is highlighted in \textbf{bold}. M represents the number of parameters in millions.}
\label{tab:ag4}
\end{table*}

\subsection{More Quantitative Analysis on Argoverse 2}
We conducted more detailed experiments on the Argoverse 2 dataset. As shown in table \ref{tab:ag4}, represents transformer-based methods, while 'y' denotes non-transformer methods. 
It is evident that current state-of-the-art trajectory prediction models struggle to balance efficiency and performance effectively.

In terms of parameter count, Tamba significantly reduces the parameter size compared to non-transformer models such as BANet (9.49M) and GANet (61.73M), achieving reductions of 52.0\% and 92.7\% respectively, while still outperforming both models. Compared to Transformer-based methods such as QCNet and MTR, Tamba demonstrates a more significant efficiency advantage. MTR has 65.78M parameters and QCNet has 7.66M parameters, while Tamba reduces the parameter count by 93.1\% and 40.7\%, respectively. Additionally, Tamba achieves 27.3 GigaOps per second, which is 40\% faster than QCNet’s 45.3 GigaOps per second. 

In terms of performance, Tamba achieves near-optimal results across almost all evaluation metrics, consistently outperforming other state-of-the-art methods. QCNet only slightly outperforms Tamba in the MR$_6$ metric. These findings further confirm Tamba’s advantage in balancing both performance and efficiency.

\section{More Quantization Results}
We visualized more detailed scene types to illustrate Tamba's trajectory predictions. As shown in Fig. \ref{fig:5}, these visualizations are based on the Argoverse 2 validation set.
(a) depicts a straight-road scenario involving multiple agents. In this scenario, Tamba accurately predicts the target agent yielding to an oncoming vehicle, with the predicted trajectory (yellow dashed line) closely aligning with the realized ground truth (orange line).
(b) illustrates a curved road with multiple agents, where Tamba's trajectory prediction is smooth and highly consistent with the ground truth.
(c) represents a more complex roundabout road scenario with multiple agents. After predicting the initial curve, Tamba correctly anticipates a potential collision with a vehicle ahead and adjusts the predicted trajectory accordingly, which aligns perfectly with the ground truth.
(d) shows a mixed scenario involving pedestrians and vehicles. Under the influence of map elements like traffic lights, pedestrians cross the road following the traffic light signals, while other agents remain stationary.
